# Supplementary material for: Do LLMs Know When to NOT Answer? Investigating Abstention Abilities of Large Language Models
Source: arXiv:2407.16221 source file (2024-09-24)
Supplement: Supplementary file 1 [file appendix_prompt.tex]

% \subsection{Sample Task Prompts}
% \label{app:task prompts}
% Task prompts ($\phi$) for the Base, Verbal Confidence and Chain of Thought (CoT) experiments are given below. All examples are taken from the MMLU dataset.

% \vspace{-2mm}

% %Task prompt - Base
% \begin{tcolorbox}[colback=gray!10!white, colframe=gray!30!white, coltitle=black, title=\footnotesize{\textbf{$\phi$ (Base)}}, width=1\columnwidth, left=2mm, right=2mm]
% \scriptsize{
% In this task, you are given an MCQ (Multiple Choice Question) based on the topic: \textbf{HIGH SCHOOL MATHEMATICS}, and you have to answer the same. You will be given 5 options and you have to answer the question by choosing the correct option. Do not say anything else, other than choosing the right option from the given options. Do not give any explanation for your answer. Take your time, think and carefully generate your answer.

% \vspace{0.2cm}
% Use the format given below to present your answer: 

% \noindent{OPTION - <NUMBER>} 

% \vspace{0.2cm}
% \textbf{Question:}  An 8.5-by-11-inch piece of paper is folded in half repeatedly (never being unfolded), each time shortening what was then the longer side. What is the length of the longest side, in inches, immediately after the second fold? Express your answer as a decimal to the nearest tenth.

% \noindent{\textbf{Options:}}

% \noindent{(1) 5.5}

% \noindent{(2) 4.5}

% \noindent{(3) 5}

% \noindent{(4) "I Don't Know/ None of the above".}

% \noindent{(5) 1}}
% \end{tcolorbox}


% \vspace{-5mm}

% %Task prompt - Verbal Confidence
% \begin{tcolorbox}[colback=gray!10!white, colframe=gray!30!white, coltitle=black, title=\footnotesize{\textbf{$\phi$ (Verbal Confidence)}}, width=1\columnwidth, left=2mm, right=2mm]
% \scriptsize{
% In this task, you are given an MCQ (Multiple Choice Question) based on the topic: \textbf{ANATOMY}, and you have to answer the same. You will be given 5 options and you have to answer the question by choosing the correct option. Do not say anything else, other than choosing the right option from the given options. Do not give any explanation for your answer. Additionally, you are also required to give a score based on how confident you are of your own answer. The score should be in the range of 1 to 5 where 1 being 'Least Confident' while 5 being 'Extremely Confident'. Take your time, think and carefully generate your answer.

% \vspace{0.2cm}
% Use the format given below to present your answer: 

% \noindent{OPTION - <NUMBER>} 

% \noindent{CONFIDENCE - <NUMBER>}

% \vspace{0.2cm}
% \textbf{Question:} Palatine shelf elevation is due to the effect of

% \noindent{\textbf{Options:}}

% \noindent{(1) changes in flexure of the developing brain.}

% \noindent{(2) a combination of these three processes.}

% \noindent{(3) hydrophilic molecules increasing turgor pressure in the palatine shelves.}

% \noindent{(4) descent of the tongue.}

% \noindent{(5) "I Don't Know/ None of the above".}}
% \end{tcolorbox}


% \vspace{-5mm}

% %Task prompt - CoT
% \begin{tcolorbox}[colback=gray!10!white, colframe=gray!30!white, coltitle=black, title=\footnotesize{\textbf{$\phi$ (CoT)}}, width=1\columnwidth, left=2mm, right=2mm]
% \scriptsize{
% In this task, you are given an MCQ (Multiple Choice Question) based on the topic: 

% \noindent{\textbf{PROFESSIONAL PSYCHOLOGY}}, and you have to answer the same. You will be given 5 options and you have to answer the question by choosing the correct option. In addition to this, you are required to verbalise your thought process that goes into, before answering the given question. You should mention each and every single point that you think of, before answering a given question. You are required to mention these points as bullet points. Take your time, think STEP BY STEP and carefully generate your answer.

% \vspace{0.2cm}
% Use the JSON format given below to present your answer: 

% \noindent{\{"CHAIN OF THOUGHT": <YOUR THOUGHT PROCESS MENTIONED IN BULLET POINTS>,}

% \noindent{"OPTION": <NUMBER>\}}

% \vspace{0.2cm}
% \textbf{Question:} The primary function of the psychology licensing board is best described as

% \noindent{\textbf{Options:}}

% \noindent{(1) protecting the public welfare.}

% \noindent{(2) "I Don't Know/ None of the above".}

% \noindent{(3) developing laws that govern the practice of psychology.}

% \noindent{(4) accrediting graduate programs in psychology.}

% \noindent{(5) providing sanctions for unethical and illegal behavior on the part of psychologists.}}
% \end{tcolorbox}




% \subsection{Question Generation Templates}
% \label{app:question generation templates}

% This section contains some of the Question generation templates used to generate the MCQs of Carnatic-QA. Specifically, the templates for tasks 1, 6 and 8 are shown. These templates belong to the Verbal Confidence, Base and CoT experimental setups, respectively and they are of standard type i.e., neither $\mathcal{AC}$ nor $\mathcal{EAC}$ is present. Note that all nine question generation templates have respective variations according to the experiment type and the Abstain clause type (Standard, $\mathcal{AC}$ or $\mathcal{EAC}$).



% %CQA-Task6-No confidence
% \begin{tcolorbox}[colback=gray!10!white, colframe=gray!30!white, coltitle=black, title=\footnotesize{\textbf{CQA - Task 6 - Standard - Base}}, width=1\columnwidth, left=2mm, right=2mm]
% \scriptsize{
% In this task, you are given a set of Arohanas and Avarohanas (also called the scales) of some Carnatic Music Ragas and you are required to identify which Arohana and Avarohana among the given set, belongs to a Melakarta raga. The Arohanas and Avarohanas in the set will be given to you as options of four, of an MCQ and you have to choose the right answer. Do not say anything else, other than choosing the right answer from the given options. Do not give any explanation for your answer.Take your time, think and carefully generate your answer.

% \vspace{0.2cm}
% Use the format given below to present your answer: 

% \noindent{OPTION - <NUMBER>} 

% \vspace{0.2cm}
% \textbf{Question:} Given the below set of Arohanas and Avarohanas of some Carnatic Music ragas, identify the Arohana and Avarohana which belongs to a Melakarta raga, by choosing the correct option.

% \noindent{\textbf{Options:}}

% \noindent{(1) 
% \textbf{Arohana:} \_   ; \textbf{Avarohana:}} \_

% \noindent{(2) 
% \textbf{Arohana:} \_   ; \textbf{Avarohana:}} \_

% \noindent{(3) 
% \textbf{Arohana:} \_   ; \textbf{Avarohana:}} \_

% \noindent{(4) 
% \textbf{Arohana:} \_   ; \textbf{Avarohana:}} \_

% \noindent{(5) "I Don’t Know/ None of the above".}

% \vspace{0.2cm}

% Note that in the above options, you are given 'I Don't Know/ None of the above' as an additional option, which can also be utilised accordingly, to generate your answer. 

% \vspace{0.2cm}

% \noindent{\textbf{Reference for understanding the Arohana and Avarohana given above:} In Carnatic music, the notations S,R1,R2,R3,G1,G2,G3,M1,M2,P,D1,
% D2,D3,N1,N2,N3,Su represent the syllables for the respective musical notes: 
% S: Shadjam, R1: Shuddha Rishabham, R2: Chatushruti Rishabham, R3: Shatshruti Rishabham, G1: Shuddha Gandharam, G2: Sadharana Gandharam, G3: Antara Gandharam, M1: Shuddha Madhyamam, M2: Prati Madhyamam, P: Panchamam, D1: Shuddha Dhaivatam, D2: Chatushruti Dhaivatam, D3: Shatshruti Dhaivatam, N1: Shuddha Nishadham, N2: Kaishiki Nishadham, N3: Kakali Nishadham, Su: Shadjam of the upper octave.}

% \vspace{0.2cm}

% \noindent{\textbf{Reference for understanding Melakarta ragas in Carnatic Music:} Melakarta ragas - They are the fundamental ragas and are 72 in number. They form the basis of the melodic structure in Carnatic Music and each one is associated with a unique set of seven swaras (musical notes). Example: Raga Kalyani.}}
% \end{tcolorbox}




% %CQA-Task1-Verbal Confidence
% \begin{tcolorbox}[colback=gray!10!white, colframe=gray!30!white, coltitle=black, title=\footnotesize{\textbf{CQA - Task 1 - Standard - Verbal Confidence}}, width=1\columnwidth, left=2mm, right=2mm]
% \scriptsize{
% In this task, you are given an Arohana and Avarohana (also called the scale) of a Carnatic Music Raga and you have to detect the name of that Raga by carefully analysing the given Arohana and Avarohana. You will be given 5 options and you have to choose the right answer. Do not say anything else, other than choosing the right answer from the given options. Do not give any explanation for your answer. Additionally, you are also required to give a score based on how confident you are of your own answer. The score should be in the range of 1 to 5 where 1 being 'Least Confident' while 5 being 'Extremely Confident'. Take your time, think and carefully generate your answer.

% \vspace{0.2cm}
% Use the format given below to present your answer: 

% \noindent{OPTION - <NUMBER>} 

% \noindent{CONFIDENCE - <NUMBER>}

% \vspace{0.2cm}
% \textbf{Arohana:} \_

% \noindent{\textbf{Avarohana:}} \_

% \noindent \textbf{Question:} Given the above Arohana and Avarohana, identify the raga name by choosing the correct option.

% \noindent{\textbf{Options:}}

% \noindent{(1) \_}

% \noindent{(2) \_}

% \noindent{(3) \_}

% \noindent{(4) \_}

% \noindent{(5) \_}

% \vspace{0.2cm}

% \noindent{\textbf{Reference for understanding the Arohana and Avarohana given above:} In Carnatic music, the notations S,R1,R2,R3,G1,G2,G3,M1,M2,P,D1,
% D2,D3,N1,N2,N3,Su represent the syllables for the respective musical notes: 
% S: Shadjam, R1: Shuddha Rishabham, R2: Chatushruti Rishabham, R3: Shatshruti Rishabham, G1: Shuddha Gandharam, G2: Sadharana Gandharam, G3: Antara Gandharam, M1: Shuddha Madhyamam, M2: Prati Madhyamam, P: Panchamam, D1: Shuddha Dhaivatam, D2: Chatushruti Dhaivatam, D3: Shatshruti Dhaivatam, N1: Shuddha Nishadham, N2: Kaishiki Nishadham, N3: Kakali Nishadham, Su: Shadjam of the upper octave}}
% \end{tcolorbox}



% %CQA-Task8-CoT
% \begin{tcolorbox}[colback=gray!10!white, colframe=gray!30!white, coltitle=black, title=\footnotesize{\textbf{CQA - Task 8 - Standard - CoT}}, width=1\columnwidth, left=2mm, right=2mm]
% \scriptsize{
% In this task, you are given the names of some Carnatic Music Ragas and you are required to identify which, among the given raga names, is a Janya raga name. The raga names will be given to you as options of four, of an MCQ and you have to choose the right answer. In addition to this, you are required to verbalise your thought process that goes into, before answering the given question. You should mention each and every single point that you think of, before answering a given question. You are required to mention these points as bullet points. Take your time, THINK STEP BY STEP and carefully generate your answer.

% \vspace{0.2cm}
% Use the JSON format given below to present your answer: 

% \noindent{\{"CHAIN OF THOUGHT": <YOUR THOUGHT PROCESS MENTIONED IN BULLET POINTS>,}

% \noindent{"OPTION": <NUMBER>\}}

% \vspace{0.2cm}
% \textbf{Question:} Given the below Carnatic Music raga names, identify the Janya raga name by choosing the correct option.

% \noindent{\textbf{Options:}}

% \noindent{(1) \_}

% \noindent{(2) \_}

% \noindent{(3) \_}

% \noindent{(4) \_}

% \noindent{(5) "I Don’t Know/ None of the above".}

% \vspace{0.2cm}

% Note that in the above options, you are given 'I Don't Know/ None of the above' as an additional option, which can also be utilised accordingly, to generate your answer. 

% \vspace{0.2cm}

% \noindent{\textbf{Reference for understanding Melakarta and Janya ragas in Carnatic Music:} Melakarta ragas - They are the fundamental ragas and are 72 in number. They form the basis of the melodic structure in Carnatic Music and each one is associated with a unique set of seven swaras (musical notes). Example: Raga Kalyani.

% Janya ragas - They are derived/ created by choosing a subset of swaras from a Melakarta raga and establishing a unique melodic structure. Example: Raga Mohana.}}
% \end{tcolorbox}




% % \begin{tcolorbox}[colback=gray!10!white, colframe=gray!30!white, coltitle=black, title=\footnotesize{\textbf{CQA - Task 5 - Answerable}}, width=1\columnwidth, left=2mm, right=2mm]
% % \small{
% % \textsc{Question:}

% % \noindent{Melakarta Raga Name: Hanumatodi}

% % \noindent{Given the above Melakarta raga name, identify it's Janya raga name by choosing the right answer from the given options.}

% % \noindent{\textsc{Options:}}

% % \noindent{\textbf{(1) Dhanyasi}}

% % \noindent{(2) Chintamani}

% % \noindent{(3) Nagadhwani}

% % \noindent{(4) Patalambari}

% % \noindent{(5) "I Don’t Know/ None of the above"}}
% % \end{tcolorbox}


% % \begin{tcolorbox}[colback=gray!10!white, colframe=gray!30!white, coltitle=black, title=\footnotesize{\textbf{CQA - Task 5 - Unanswerable}}, width=1\columnwidth, left=2mm, right=2mm]
% % \small{
% % \textsc{Question:} 

% % \noindent{Melakarta Raga Name: Naganandini}

% % \noindent{Given the above Melakarta raga name, identify it's Janya raga name by choosing the right answer from the given options.}

% % \noindent{\textsc{Options:}}

% % \noindent{(1) Madhavamanohari}

% % \noindent{\textbf{(2) "I Don’t Know/ None of the above"}}

% % \noindent{(3) Gambheeranattai}

% % \noindent{(4) Madhavamanohari}

% % \noindent{(5) Mohana}}
% % \end{tcolorbox}
